# Supplementary material for: RABBIT: A Robot-Assisted Bed Bathing System with Multimodal Perception and Integrated Compliance
Source: arXiv:2401.15159 source file (2025-04-23)
Supplement: Supplementary file 1 [file appendix.tex]

To support building a strong evidence base in HRI, and encourage future reproducibility of published work, all submissions involving studies with human participants should clearly outline their methodology regardless of the theme they are submitted to, including:

Ethical aspects considered and clearance obtained where appropriate (c.f., Geiskkovitch et al. 2016, Sections 5.2, 5.4)
Participant demographics and sampling approach, e.g. gender, ethnicity, etc. (c.f., de Graaf 2017, Section 2.3, recommendations in Schlesinger et al., 2017)
Data collection and analysis methods (c.f., Paepcke and Takayama 2010, Section V)
Study environment and context (c.f., Short et al. 2018, Section 3.5)
If a Wizard-of-Oz paradigm was used, a detailed description of the robot, wizard, user, etc. (c.f., Riek 2012, Table 2)
If a robot was used, a detailed description of the platform, its level of autonomy, capabilities, etc. (c.f., Beer et al. 2014, Figure 5)
